# Supplementary material for: All-electron machine-learned orbital-free density functional for periodic CHNO systems
Source: arXiv:2610.17975 source file (2026-10-13)
Supplement: Supplementary file 2 [file numbers.tex]

\newcommand{\CommonCount}{516}
\newcommand{\RankingCommonCount}{465}
\newcommand{\ShiftMedian}{0.43}
\newcommand{\ShiftMean}{2.78}
\newcommand{\ModelOldMAE}{1.69}
\newcommand{\ModelOldMedian}{0.98}
\newcommand{\StepLargeCount}{5}
\newcommand{\ChTwoPairMaximum}{0.20}
